# Supplementary material for: Complex networks as an emerging property of hierarchical preferential attachment
Source: arXiv:1312.0171 source file (2015-12-10)
Supplement: Supplementary file 1 [file LHD13_SI_HPA.pdf]

# **Complex networks are an emerging property of hierarchical preferential attachment**

## **Supporting Information**

Laurent Hébert-Dufresne, Edward Lawrence, Antoine Allard, Jean-Gabriel Young and Louis J. Dubé

<http://dynamica.phy.ulaval.ca/>

*Département de Physique, de Génie Physique et d'Optique  
Université Laval, Québec, Québec, Canada G1V0A6*

## **Contents**

|          |                                                  |          |
|----------|--------------------------------------------------|----------|
| <b>1</b> | <b>Solving a preferential attachment process</b> | <b>2</b> |
| <b>2</b> | <b>On structure sizes in HPA</b>                 | <b>2</b> |
| <b>3</b> | <b>On node memberships in HPA</b>                | <b>3</b> |
| <b>4</b> | <b>Multiple scale independence</b>               | <b>4</b> |
| <b>5</b> | <b>On the fractality of projected networks</b>   | <b>4</b> |

## 1 Solving a preferential attachment process

We study any process where the evolution of the number of elements  $N_s(t)$  with share  $s$  at time  $t$  follow a master equation of the type:

$$N_s(t + \Delta t) = N_s(t) + B\delta_{s,1} + \frac{G}{(B+G)t} [(s-1)N_{s-1}(t) - sN_s(t)] . \quad (1.1)$$

Since  $B$  is the birth probability, the evolution of the normalized distribution  $\{n_s(t)\}$  can be obtained by replacing  $N_s(t)$  by  $Bt n_s(t)$ :

$$B(t + \Delta t) n_s(t + \Delta t) = Bt n_s(t) + B\delta_{s,1} + \frac{GB}{B+G} [(s-1)n_{s-1}(t) - sn_s(t)] . \quad (1.2)$$

Since  $\Delta t$  is an arbitrary time step, and  $B$  and  $G$  are just as arbitrary (only both smaller than 1), we can use an equivalent process in continuous time by using  $\Delta t \rightarrow dt$ ,

$$B(t + dt) n_s(t + dt) = Bt n_s(t) + dt \left\{ \frac{GB}{B+G} [(s-1)n_{s-1}(t) - sn_s(t)] + B\delta_{s,1} \right\} , \quad (1.3)$$

from which the following set of ordinary differential equations is obtained:

$$\lim_{dt \rightarrow 0} \frac{(t + dt) n_s(t + dt) - t n_s(t)}{dt} = \frac{d}{dt} [t n_s(t)] = \frac{G}{B+G} [(s-1)n_{s-1}(t) - sn_s(t)] + \delta_{s,1} . \quad (1.4)$$

Solving at statistical equilibrium, i.e.  $n_s(t) = n_s^*$  such that  $\frac{d}{dt} n_s(t) = 0 \forall s$  yields

$$\left(1 + s \frac{G}{G+B}\right) n_s^* = \frac{G}{G+B} (s-1) n_{s-1}^* + \delta_{s,1} \quad (1.5)$$

or more directly

$$n_s^* = \frac{\prod_{m=1}^{s-1} \frac{G}{G+B} m}{\prod_{m=1}^s \left(1 + m \frac{G}{G+B}\right)} . \quad (1.6)$$

Assuming a scale-free behaviour for  $s \rightarrow \infty$ , this steady state can be shown to scale as

$$\lim_{s \rightarrow \infty} \frac{n_{s+1}^*}{n_s^*} = \left(\frac{s+1}{s}\right)^{-\gamma} \quad \text{where } \gamma = 2 + \frac{B}{G} . \quad (1.7)$$

## 2 On structure sizes in HPA

In the main text, structure sizes were approximated to follow simple equations under the general form of Eq. (1.1). However, while this is exact for the first structural level, the probability that a structure of size  $n$  in level 2 will depend on the size  $m$  of the level 1 structure in which it is nested. Mathematically, level 1 evolves according to

$$S_{1,n}(t + \Delta t) = S_{1,n}(t) + p_1 \delta_{n,1} + \frac{(1-p_1)p_2}{[p_1 + (1-p_1)p_2]t} [(n-1)S_{1,n-1}(t) - nS_{1,n}(t)] \quad (2.1)$$

and level 2 follows

$$\begin{aligned} S_{2,n,m}(t + \Delta t) = & S_{2,n,m}(t) + \frac{(1-p_1)mS_{1,m}(t)}{[p_1 + (1-p_1)p_2]t} \left\{ (1-p_2)p_3 \frac{(n-1)S_{2,n-1,m}(t) - nS_{2,n,m}(t)}{\sum_i i S_{2,i,m}(t)} - p_2 \frac{S_{2,n,m}(t)}{S_{1,m}(t)} \right\} \\ & + \frac{(1-p_1)(1-p_2)p_3}{[p_1 + (1-p_1)p_2]t} \sum_{m'} \frac{(n-1)S_{2,n-1,m'}(t) - nS_{2,n,m'}(t)}{\langle n \rangle_{2,m'}} + p_1 \delta_{n,1} \delta_{m,1} \end{aligned} \quad (2.2)$$

where  $S_{2,n,m}(t)$  is the number of level 2 structure which are of size  $n$  and nested in level 1 structure of size  $m$  and  $\sum_i i S_{2,i,m}(t)/m S_{1,m}(t) = \langle n \rangle_{2,m}$  is the average value of these sizes  $n$  for a given  $m$ .

To obtain a master equation following the form of Eq. (1.1) one must sum over all  $m$  while assuming  $\langle n \rangle_{2,m} = \langle n \rangle_2 \forall m$ , such that  $[p_1 + (1 - p_1)p_2]t \cdot \langle n \rangle_2 = [p_1 + (1 - p_1)p_2 + (1 - p_1)(1 - p_2)p_3]t$ ; yielding the form presented directly in the main text by considering uncorrelated levels of organization. These approximations are the source of the error observed in the mean-field description of distribution  $S_{k,n}(t)$  for  $k > 1$  and are progressively worse for higher  $k$  (lower structural levels). The progression in error is essentially caused by the fact that a strict description of the third level, for instance, should not only be given in terms of  $S_{3,n,m}(t)$ , but of  $S_{3,n,m,l}(t)$  describing the number of level 3 structures of size  $n$  nested in level 2 structures of size  $m$  themselves nested in level 1 structures of size  $l$ .

### 3 On node memberships in HPA

We are interested in obtaining the thermodynamic limit, i.e. when  $t \rightarrow \infty$ , for the distribution of node memberships at level  $k$  (the distribution of level  $k$  structures in which a given color appears). In the main text, we solved the problem of logical constraints on node memberships by introducing a biased set of probabilities  $\{q'_i\}$ :

$$q'_k(t) = q_k + \frac{S_{k-1,1}(t)}{\sum_n n \cdot S_{k-1,n}(t)} (1 - q_k) . \quad (3.1)$$

Within our mean-field description of time evolution, these probabilities can be explicitly calculated at each time step using the current size distribution at level  $k - 1$ . In the thermodynamic limit, we can instead use the steady-state distributions described by Eq. (1.6). Doing so yields

$$q'_k = q_k + \frac{S_{k-1,1}^*}{\sum_n n \cdot S_{k-1,n}^*} (1 - q_k) = q_k + \frac{G_{k-1}^{(S)} + B_{k-1}^{(S)}}{2G_{k-1}^{(S)} + B_{k-1}^{(S)}} \frac{1 - q_k}{\langle n \rangle_{k-1}} \quad (3.2)$$

where the average size  $\langle n \rangle_{k-1}$  is straightforwardly calculated as the ratio of total events to birth events:

$$\langle n \rangle_{k-1} = \frac{[G_{k-1}^{(S)} + B_{k-1}^{(S)}]t}{(B_{k-1}^{(S)})t} \quad (3.3)$$

such that

$$q'_k = q_k + \frac{(1 - q_k) B_{k-1}^{(S)}}{2G_{k-1}^{(S)} + B_{k-1}^{(S)}} . \quad (3.4)$$

This set of probabilities is then used to obtain master equations following Eq. (1.1) by assuming that memberships and structure sizes are uncorrelated, meaning that a node with  $m$  memberships at level  $k$ , has memberships in nested in level  $k - 1$  structures following the same distribution as those of a node with  $m'$  memberships. Such that an event at level  $k$  is  $m/m'$  times more likely to involve the first node and not the latter, notwithstanding whether these memberships are within the correct structure or not. Similarly, when a structure is created at level  $k - 1$ , we are effectively adding a membership at level  $k$ . Assuming that the node with  $m$  memberships at level  $k$  has  $m/m'$  more memberships at level  $k - 1$  than the node with  $m'$  memberships, these events affect the distribution in the same manner than regular growth events.

## 4 Multiple scale independence

We showed how we can only approximately follow the time evolution of the size distributions. However, we can mathematically derive the scale exponents in the thermodynamic limit  $t \rightarrow \infty$ . In the main text, we found the general scaling exponent for the size distribution of level  $k$  structures and, using the steady-state value of the corrected probabilities, we also found the scaling exponent for node memberships.

When looking at projected properties of a hierarchical system, for instance the degree distribution of the resulting network, we can compose the membership and size distributions of the lowest level (where links are created) and deduce the resulting scaling exponent. As done in [Hébert-Dufresne *et al.*, Phys. Rev. E, **85**, 026108 (2012)], the idea is to define the following *probability generating functions* (pgf):

$$S(x, t) = \sum_n S_{d,n}(t) x^n \quad \text{and} \quad \mathcal{N}(x, t) = \sum_m N_{d,m}(t) x^m. \quad (4.1)$$

As a community of size  $n$  implies  $n - 1$  links for each node, this last distribution can be generated by

$$S_l(x, t) = \frac{\frac{d}{dx} S(x, t)}{\frac{d}{dx} S(x, t)|_{x=1}} = \frac{\sum_n S_{d,n}(t) n x^{n-1}}{\sum_n S_{d,n}(t) n}. \quad (4.2)$$

The degree distribution is then generated by a pgf  $\mathcal{D}(x, t)$  combining the distribution of memberships  $m$  and of link obtained from each of this membership:

$$\mathcal{D}(x, t) = \mathcal{N}(S_l(x, t), t), \quad (4.3)$$

which simply scales as the slowest falling function between  $\mathcal{N}(x, t)$  and  $S_l(x, t)$ . The scale exponent of the degree distribution is thus given by

$$\min \left[ \gamma_d^{(N)}, \gamma_d^{(S)} - 1 \right]. \quad (4.4)$$

The same method could of course be used to determine the scaling of other projections; e.g., network of companies sharing or having shared at least one producer).

## 5 On the fractality of projected networks

As shown in the main text, HPA can produce both fractal and non-fractal networks. As the definition of network fractality is somewhat ambiguous, so is the distinction between set of HPA parameters leading to fractality or not. That being said, a rule of thumb can be established.

The dimensionality of a network is analyzed through standard box-counting: boxes of sizes  $r$  cover groups of nodes all within a distance  $r - 1$  or less of one another (the distance being measured in number of links). Fractal networks are characterized by a box-counting dimension  $d_b$  governing how many boxes of size  $r$ ,  $N_b(r)$ , are needed to cover all nodes. This relation takes the form  $N_b(r) \propto r^{-d_b}$ .

Most models of stochastic network growth produce networks with very low mean shortest paths, low clustering and no long-range correlations. Consequently, the number of boxes needed to cover the whole network falls very rapidly. In HPA, we can control the way boxes cover the network since the distance between higher structural level is directly influenced by the memberships at this level. Hence, HPA can generate networks that are robust to box covering (i.e. such that  $N_b(r)$  falls slower with regards to  $r$ ) if higher structural levels feature less nodes that act as bridges between structures and levels. For example, in Supp. Fig. 1, only nodes 1, 2 and 3 can be used by boxes to move from one level to the other (from cities to countries, here illustrated as an inverted tree).

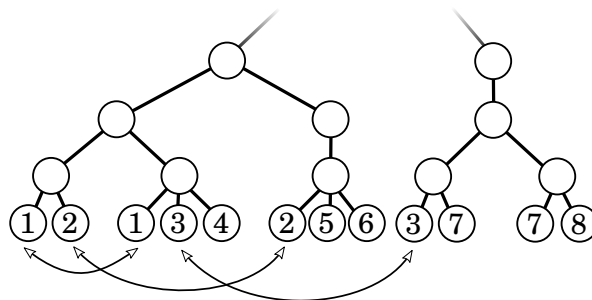

Supporting Figure 1: Example of how nodes act as bridges between structures.

Supporting Table 1: Parameters used in the case study of fractal behaviour.

| Network | p                 | q                |
|---------|-------------------|------------------|
| A       | [0.1, 0.2, 0.3]   | [0.69, 0.9, 0.1] |
| B       | [0.01, 0.02, 0.3] | [0.95, 0.8, 0.3] |

More precisely, let us consider two different networks: A and B, built using the parameters given in Supp. Table 1. Roughly speaking, in network A, level 2 structures contain on average two level 3 structures whereas nodes belong to over 4 level 3 structures. Therefore, a single node typically grants access to all level 3 structures contained within any of its level 2 structure, such that a box covering at least *part* of a level 2 structure typically covers *all* of it. The network is thus easily invaded as higher levels are not any harder to navigate.

In contrast, level 2 structures of network B contain on average eleven level 3 structures. An average node may be found within four level 3 structures, so that even a single average level 2 structure may have nodes at a distance greater than three steps. The network is thus harder to cover and can be expected to be much more robust to box-covering. Our intuition is confirmed in Supp. Fig. 2. As a general rule of thumb, we found that to feature *measurable* network self-similarity the average size of a structure (at level  $x$ ) had to be at least greater than the memberships of a node at the lower level (at level  $x + 1$ ).

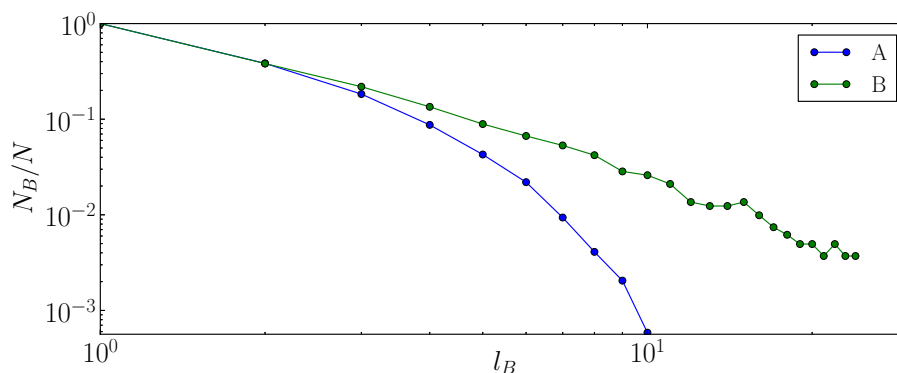

Supporting Figure 2: Box-covering results of the networks presented in the case study of (non-)fractal behaviour.
